# Supplementary material for: Confidence Estimation in Automatic Short Answer Grading with LLMs
Source: arXiv:2605.00200 source file (2026-05-13)
Supplement: Supplementary file 1 [file 08appendix.tex]

% \section{Prompts for Verbalizing-Based Confidence Estimation}
% \label{app:model_conf}

% %\subsection{Verbalizing-based Confidence}

% %Following \cite{tian2023just}, 
% We employ the following prompts for the verbalizing-based confidence estimation method:

% \smallskip
% \noindent\rule{\linewidth}{0.3pt}

% \begin{raggedright}
% \textbf{System prompt:} 

% You are a teacher grading short student responses. Classify the student’s answer as either correct (1) or incorrect (0). Reason internally about your decision, but do not include any explanation in the output. Report your confidence as a probability between 0 and~1. Answer exclusively in the following JSON format (no extra text): \\
% \{ \\
%   \hspace{5mm} "category": 0, \\
%   \hspace{5mm} "probability": 0.6 \\
% \}

% \noindent\rule{\linewidth}{0.3pt}

% \textbf{User prompt:} 

% Classify the student’s answer as correct (1) or incorrect (0). \\
% The question is: [Question] \\
% The reference answer is: [Reference\_answer] \\
% The student answer is: [Student\_answer]
% \end{raggedright}

% \noindent\rule{\linewidth}{0.3pt}


% \subsection{Latent-based Confidence}

% Based on \cite{kadavath2022languagemodelsmostlyknow}, given an input prompt prefix \(x\) and a set of candidate labels \(\mathcal{Y}\), we compute the conditional log-likelihood \(\log p(y \mid x)\) for each label \(y \in \mathcal{Y}\). These label-wise log-likelihoods are normalized across all candidates using a softmax function, and the latent confidence is defined as the normalized score assigned to the predicted label $\hat{y}$:
% \[
% s^{\text{lat}}
% = \frac{\exp\!\left(\log p(\hat{y} \mid x)\right)}
% {\sum_{y \in \mathcal{Y}} \exp\!\left(\log p(y \mid x)\right)}=\frac{ p(\hat{y} \mid x)}
% {\sum_{y \in \mathcal{Y}} p(y \mid x)}.
% \]


% \subsection{Consistency-based Confidence}

% Given an input prompt, the model is sampled multiple times under varying temperature settings, yielding a set of predicted labels \(\{ \hat{y}_1, \ldots, \hat{y}_N \}\). Following \cite{xiong2023can}, the consistency confidence for the predicted label $\hat{y}$ is defined as
% \[
% s^{\text{cons}} = \frac{1}{N} \sum_{i=1}^{N} \mathbb{I}(\hat{y}_i = \hat{y}),
% \]
% where \(\mathbb{I}(\cdot)\) denotes the indicator function. The resulting value corresponds to the empirical frequency with which the label is produced across valid sampled generations and is used as the consistency-based confidence score.

% \subsection{Unifying confidence orientation}

% All confidence scores are transformed to represent the LLM’s confidence that a student response is correct. Let $\hat{y}_i \in \{0,1\}$ denote the LLM prediction for response $x_i$, and let $s_i' \in [0,1]$ be a raw confidence signal. To ensure a consistent interpretation across predictions, we define the oriented confidence score as
% \[
% s_i =
% \begin{cases}
% s_i', & \text{if } \hat{y}_i = 1,\\
% 1 - s_i', & \text{if } \hat{y}_i = 0.
% \end{cases}
% \]
% We apply this transformation to the three model-level confidence signals.


% \section{SHAP-based feature attribution analysis}
% \label{app:feature_im}

% Table~\ref{tab:feat_importanc} reports the permutation feature importance \cite{10.1093/bioinformatics/btq134} of the individual components used in the hybrid confidence model incorporating aleatoric uncertainty. Consistency-based confidence contributes most strongly to the fused score, followed by the dataset-derived aleatoric uncertainty proxy, highlighting the importance of explicitly modeling response ambiguity. Input text length also exhibits substantial importance, suggesting that response verbosity carries informative signals related to uncertainty. In contrast, verbalizing and latent confidence scores contribute less, with latent confidence showing the lowest importance.

% \begin{table}
% \centering
% \caption{Feature importance analysis for hybrid confidence models with aleatoric uncertainty. Importance values are reported as mean $\pm$ standard deviation across runs.}
% \label{tab:feat_importanc}
% \begin{tabular}{p{6.2cm}c}
% % \toprule\\
% \midrule
% \textbf{Feature} & \textbf{Importance} \\
% \midrule
% consistency-based confidence  & 0.207 $\pm$ 0.014 \\
% aleatronic uncertainty        & 0.174 $\pm$ 0.011  \\
% input text length            & 0.161 $\pm$ 0.013  \\
% verbalizing-based confidence  & 0.154 $\pm$ 0.011 \\
% latent-based confidence      & 0.110 $\pm$ 0.009  \\
% \midrule
% % \multicolumn{3}{c}{\textbf{Hybrid model without aleatoric uncertainty}} \\
% % \midrule
% % \textbf{Feature} & \textbf{Importance (Mean)} & \textbf{Importance (Std.)} \\
% % \midrule
% % verbalizing-based confidence  & 0.230 & 0.017 \\
% % latent-based confidence    & 0.212 & 0.015 \\
% % input text length           & 0.166 & 0.010 \\
% % generated text length  & 0.152 & 0.011 \\
% % consistency-based confidence  & 0.112 & 0.008 \\
% \bottomrule
% \end{tabular}
% \end{table}



% As shown in Fig. \ref{plt:shal}, higher values of consistency and verbalizing-based confidence systematically increase the predicted hybrid confidence, whereas low values of these signals reduce it. In contrast, dataset-derived aleatoric uncertainty exhibits a strong inverse relationship with confidence. High aleatoric uncertainty suppresses confidence estimates, indicating that the model down-weights confidence for semantically ambiguous responses. Input text length shows a weaker, non-monotonic effect. Medium-length responses tend to increase predicted confidence, whereas very short responses reduce it and very long responses exhibit little influence. Finally, latent-based confidence has the smallest overall impact, suggesting that internal token-level signals play a secondary role in the hybrid model.

% \begin{figure}
% \centering
% \includegraphics[width=\linewidth]{plots/shap_hybrid.pdf}
% \caption{SHAP summary plot showing feature importance and directional effects in the hybrid confidence model incorporating aleatoric uncertainty. Colors denote feature values and SHAP values indicate each feature’s contribution to the predicted confidence. Features are ordered by mean absolute SHAP value.}
% \label{plt:shal}
% \end{figure}
